# Supplementary material for: Open-world Semi-supervised Generalized Relation Discovery Aligned in a Real-world Setting
Source: arXiv:2305.13533 source file (2023-11-01)
Supplement: Supplementary file 1 [file _DEPRECATED_a2_data_splits.tex]

%%%%%%%%%%%%%%%%%%%%%%%%%%%%%%%%%%%%%%%%%%
%%% DATA SPLITS %%%%%%%%%%%%%%%%%%%%%%%%%%%
%%%%%%%%%%%%%%%%%%%%%%%%%%%%%%%%%%%%%%%%%%
\subsection{Dataset splits}\label{sec:appendix_data_splits}
% We report the steps used to create the data splits of labeled and unlabeled data to facilitate the recreation of our experiments or to construct a similar setting for a different NLP task. 

% We first bin all instances by relation class to construct our data splits and order the bins by size. Then, given $n$ total relation classes in a dataset $D$, we select the top $\lfloor n/2 \rfloor$ most frequent classes for the set of known classes and place the remaining classes in the set of novel classes. 

% We then construct the labeled dataset by randomly selecting 85\% of instances from known classes. The remaining 15\% of instances of known classes are combined with all the instances of novel classes to create the unlabeled dataset. The \textit{no relation} class is considered a known, negative class for all settings with hard-negatives. See \ref{fig:data_splits_visual} for statistics on dataset splits.

% Note that we intentionally do not create a development set from unlabeled data to mimic real-world data that is unlabeled. A development set can easily be created from labeled data, as needed. 

% Special treatment is needed for FewRel dataset since it is a uniform dataset without entity type information. In order to obtain the true distribution of relation classes as they appear in real-word data, we obtain class frequency information directly from Wikipedia by aggregating counts of each relationship. 


% Furthermore, FewRel does not come with annotated hard-negatives (e.g., the ``no relation'' class). To better simulate real-world data, we augment the FewRel dataset with hard-negatives from ReTACRED. 


 % We resolve entity type information via the method described in Appendix \ref{sec:appendix_fewrel_types}.
% \begin{table}[ht]
% \centering
% \begin{adjustbox}{max width=0.48\textwidth}
% \begin{tabular}{| l | c | c |}
% \hline
%     & \textbf{Instances of Known Classes} & \textbf{Instances of Novel classes} \\ \hline 
% \textbf{Labeled data }  & 85\%          & 0\% \\ \hline
% \textbf{Unlabeled data} & 15\%          & 100\% \\ \hline
% \end{tabular}
% \end{adjustbox}
% \caption{Given $n$ total classes in a dataset, the set of known classes are the top $\lfloor n/2 \rfloor$ most frequent classes. All other classes are placed into the set of novel classes. Labeled data consists of a random selection of 85\% of all instances of known classes while unlabeled data contains 15\% of instances of known classes and 100\% of the instances of novel classes.}
% \label{tab:data_splits}
% \end{table}

% \begin{figure*}[ht]
%     \centering
%     \includegraphics[width=1\textwidth]{images/data_splits_and_table.pdf}
%     \caption{Data splits used for all experiments in our Generalized Relation Discovery setting. Given $n$ total classes in a dataset, the set of known classes are the top $\lfloor n/2 \rfloor$ most frequent classes. All other classes are placed into the set of novel classes. Labeled data consists of a random selection of 85\% of all instances of known classes while unlabeled data contains 15\% of instances of known classes and 100\% of the instances of novel classes (*numbers do not include hard-negatives, \textsuperscript{\dag}FewRel has no annotated hard-negatives so we augment FewRel using hard-negatives from ReTACRED).}
%     \label{fig:data_splits_visual}
% \end{figure*}


% \begin{table}[ht]
% \centering
% \begin{adjustbox}{max width=0.48\textwidth}
% \begin{tabular}{|l|c|c|c|c|c|}
% \hline
% \textbf{Dataset}  & \textbf{\begin{tabular}[c]{@{}c@{}}\# Known\\ Classes\end{tabular}} & \textbf{\begin{tabular}[c]{@{}c@{}}\# Novel\\ Classes\end{tabular}} & \textbf{\begin{tabular}[c]{@{}c@{}}\# Hard\\ Negatives\end{tabular}} & \textbf{\begin{tabular}[c]{@{}c@{}}\# Labeled \\ Instances\end{tabular}} & \textbf{\begin{tabular}[c]{@{}c@{}}\# Unlabeled ($n$ known, $n$ novel) \\ Instances\end{tabular}} \\ \hline
% \textbf{ReTACRED} & 19  & 20  & 57,777  & 25,478    & 8,212 (4474, 3738) \\ \hline
% \textbf{TACRED}   & 20  & 21  & 84,491  & 15,388    & 6,385 (2865, 3520) \\ \hline
% \textbf{FewRel}   & 40  & 40  & $0^*$       & 23,626    & 32,374 (4374, 28000) \\ \hline
% \end{tabular}
% \end{adjustbox}
% \caption{Statistics on labeled and unlabeled data splits for each dataset used in this study. *We augment FewRel with hard-negatived from ReTACRED since FewRel does not include hard-negatives.}
% \label{tab:dataset_stats}
% \end{table}
